# Supplementary material for: CrossVideoMAE: Self-Supervised Image-Video Representation Learning with Masked Autoencoders
Source: arXiv:2502.07811 source file (2025-02-08)
Supplement: Supplementary file 1 [file supplementary.tex]

\documentclass[10pt,twocolumn,letterpaper]{article}

\usepackage[review]{cvpr}      %

\input{preamble}

\definecolor{cvprblue}{rgb}{0.21,0.49,0.74}
\usepackage[pagebackref,breaklinks,colorlinks,allcolors=cvprblue]{hyperref}
\usepackage{multirow}
\usepackage{colortbl}
\usepackage{pifont}

\title{CrossVideoMAE: Self-Supervised Image-Video Contrastive Spatiotemporal and Semantic Representation Learning}

\author{First Author\\
Institution1\\
Institution1 address\\
{\tt\small firstauthor@i1.org}
\and
Second Author\\
Institution2\\
First line of institution2 address\\
{\tt\small secondauthor@i2.org}
}

\begin{document}
\maketitle

\input{sec_v2/X_suppl}

{
    \small
    \bibliographystyle{ieeenat_fullname}
    \bibliography{main}
}

\end{document}
